# Supplementary material for: FastHare: Fast Hamiltonian Reduction for Large-scale Quantum Annealing
Source: arXiv:2205.05004 source file (2022-05-10)
Supplement: Supplementary file 1 [file appendix.tex]

% !TEX root = main.tex

%\section{Neighbor compression algorithm}
%\label{app:alg-compress2}
%
%\begin{algorithm}[H]
%	%	 
%	\small 
%	\SetKwInOut{Input}{Input}
%	\SetKwInOut{Output}{Output}	
%	\SetKwFor{Event}{}{}{}	
%	\Input{A graph $G = (V,E,w)$.}
%	\Output{A serie of compression $(G_1,\mapf_1,F_1),(G_2,\mapf_2,F_2),\cdots$.}
%	$G_0 = G$\\
%	$i = 0$\\
%	\Repeat{$\mathcal{X} = \emptyset$ and $X = \emptyset$}{
%		$i = i + 1$\\
%		$((\mathcal{X},\mathcal{R}),(X,F)) = \flipsetn(G_{i-1})$\\
%		\eIf{$\mathcal{X} \ne \emptyset$}{$(G_i,\mapf_i,F_i) = \compressm(G_{i-1},\mathcal{X},\mathcal{R})$}{
%			\lIf{$X \ne \emptyset$}{$(G_i,\mapf_i,F_i) = \compress(G_{i-1},X,F)$}
%		}
%	}
%	Return  $(G_1,\mapf_1,F_1),(G_2,\mapf_2,F_2),\cdots,(G_i,\mapf_i,F_i)$
%	\caption{Neighbor compression.}
%	\label{alg:compress2}
%	% 
%\end{algorithm}
%
%\section{Compression algorithm}
%\label{app:alg-compress}
%\begin{algorithm}[H]
%	%	 
%	\small 
%	\SetKwInOut{Input}{Input}
%	\SetKwInOut{Output}{Output}	
%	\SetKwFor{Event}{}{}{}	
%	\Input{A graph $G = (V,E,w)$, a parameter $k$.}
%	\Output{A serie of compression $(G_1,\mapf_1,F_1),(G_2,\mapf_2,F_2),\cdots$.}
%	$G_0 = G$\\
%	$i = 0$\\
%	\Repeat{$\mathcal{X} = \emptyset$ and $X = \emptyset$}{
%		$i = i + 1$\\
%		$((\mathcal{X},\mathcal{R}),(X,F)) = \findset(G_{i-1},k)$\\
%		\eIf{$\mathcal{X} \ne \emptyset$}{$(G_i,\mapf_i,F_i) = \compressm(G_{i-1},\mathcal{X},\mathcal{R})$}{
%			\lIf{$X \ne \emptyset$}{$(G_i,\mapf_i,F_i) = \compress(G_{i-1},X,F)$}
%		}
%	}
%	Return  $(G_1,\mapf_1,F_1),(G_2,\mapf_2,F_2),\cdots,(G_i,\mapf_i,F_i)$
%	
%	\caption{Compression.}
%	\label{alg:compression}
%	% 
%\end{algorithm}
